# Supplementary material for: Robust Object Modeling for Visual Tracking
Source: arXiv:2308.05140 source file (2023-08-09)
Supplement: Supplementary file 1 [file vis_supple.pdf]

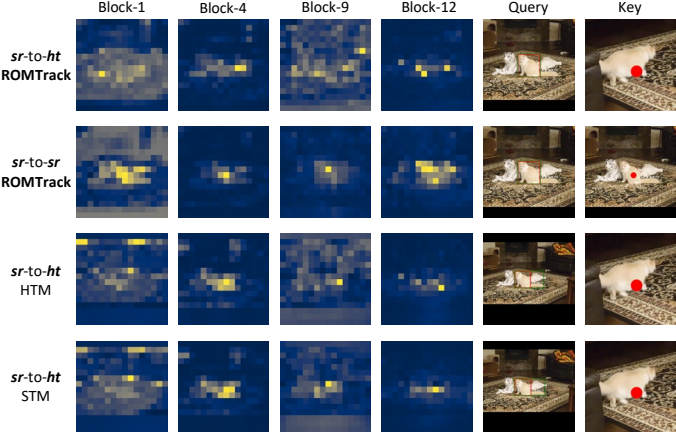

SeqName: cat-3

FrameID: 3566

Block-1

Block-4

Block-9

Block-12

Query

Feature of *sr*  
ROMTrack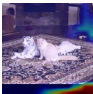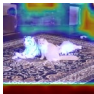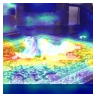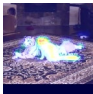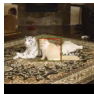Feature of *sr*  
HTM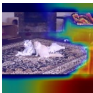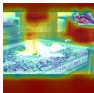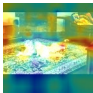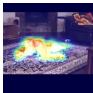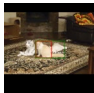Feature of *sr*  
STM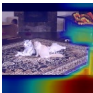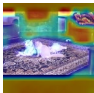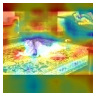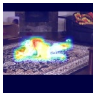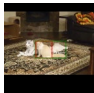

SeqName: cat-3

FrameID: 3566

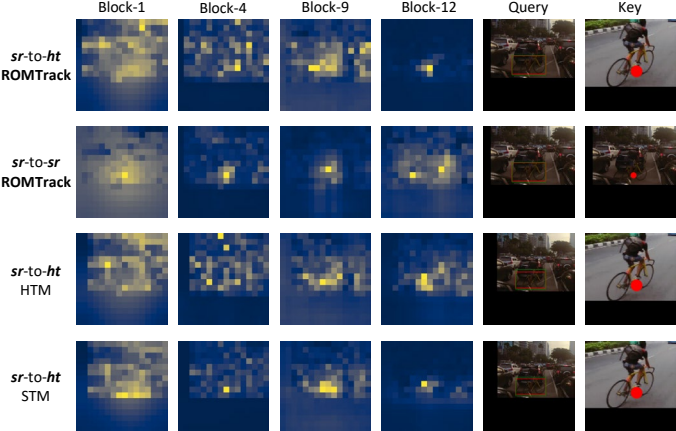

SeqName: bicycle-9

FrameID: 2613

Block-1

Block-4

Block-9

Block-12

Query

Feature of *sr*  
ROMTrack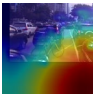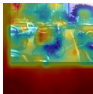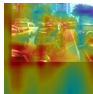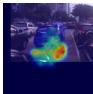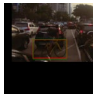Feature of *sr*  
HTM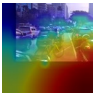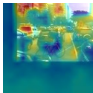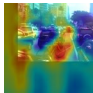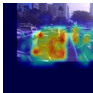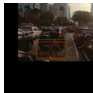Feature of *sr*  
STM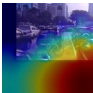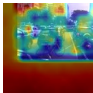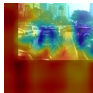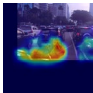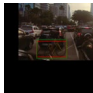

SeqName: bicycle-9

FrameID: 2613

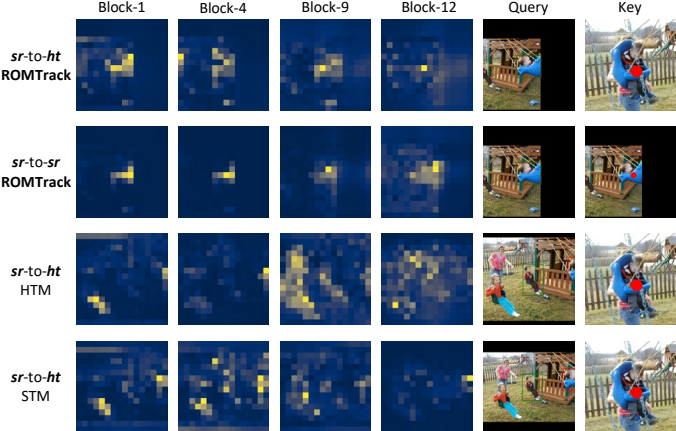

SeqName: swing-10

FrameID: 184

Block-1

Block-4

Block-9

Block-12

Query

Feature of *sr*  
ROMTrack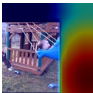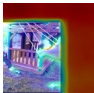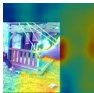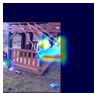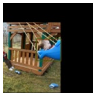Feature of *sr*  
HTM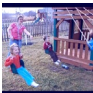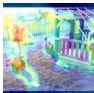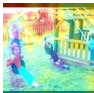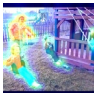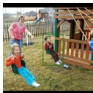Feature of *sr*  
STM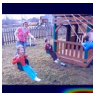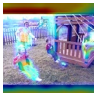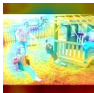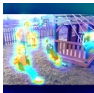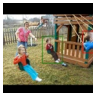

SeqName: swing-10

FrameID: 184

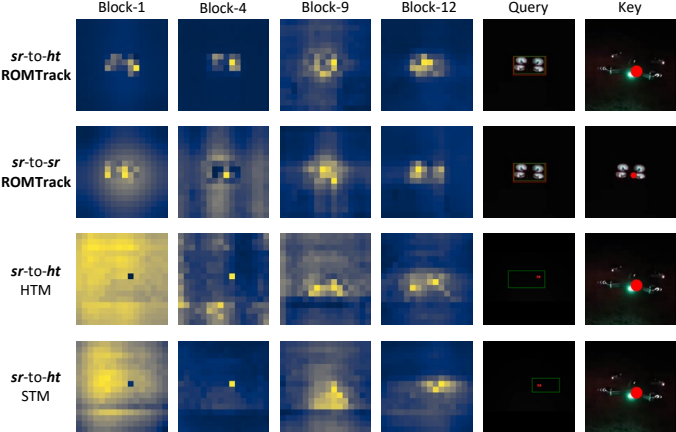

SeqName: drone-2

FrameID: 1741

Block-1

Block-4

Block-9

Block-12

Query

Feature of *sr*  
ROMTrack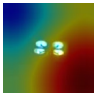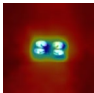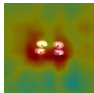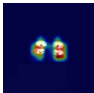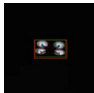Feature of *sr*  
HTM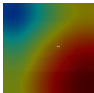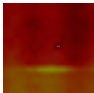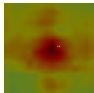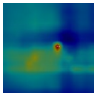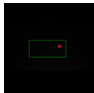Feature of *sr*  
STM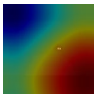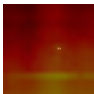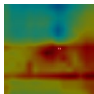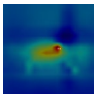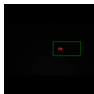

SeqName: drone-2

FrameID: 1741
